# Supplementary material for: Neuralangelo: High-Fidelity Neural Surface Reconstruction
Source: arXiv:2306.03092 source file (2023-06-12)
Supplement: Supplementary file 1 [file appendix_nvidia_jhu.pdf]

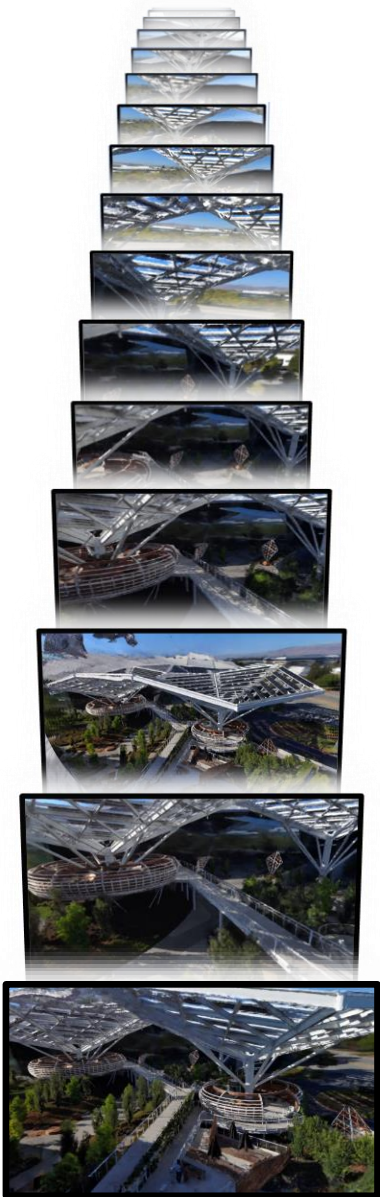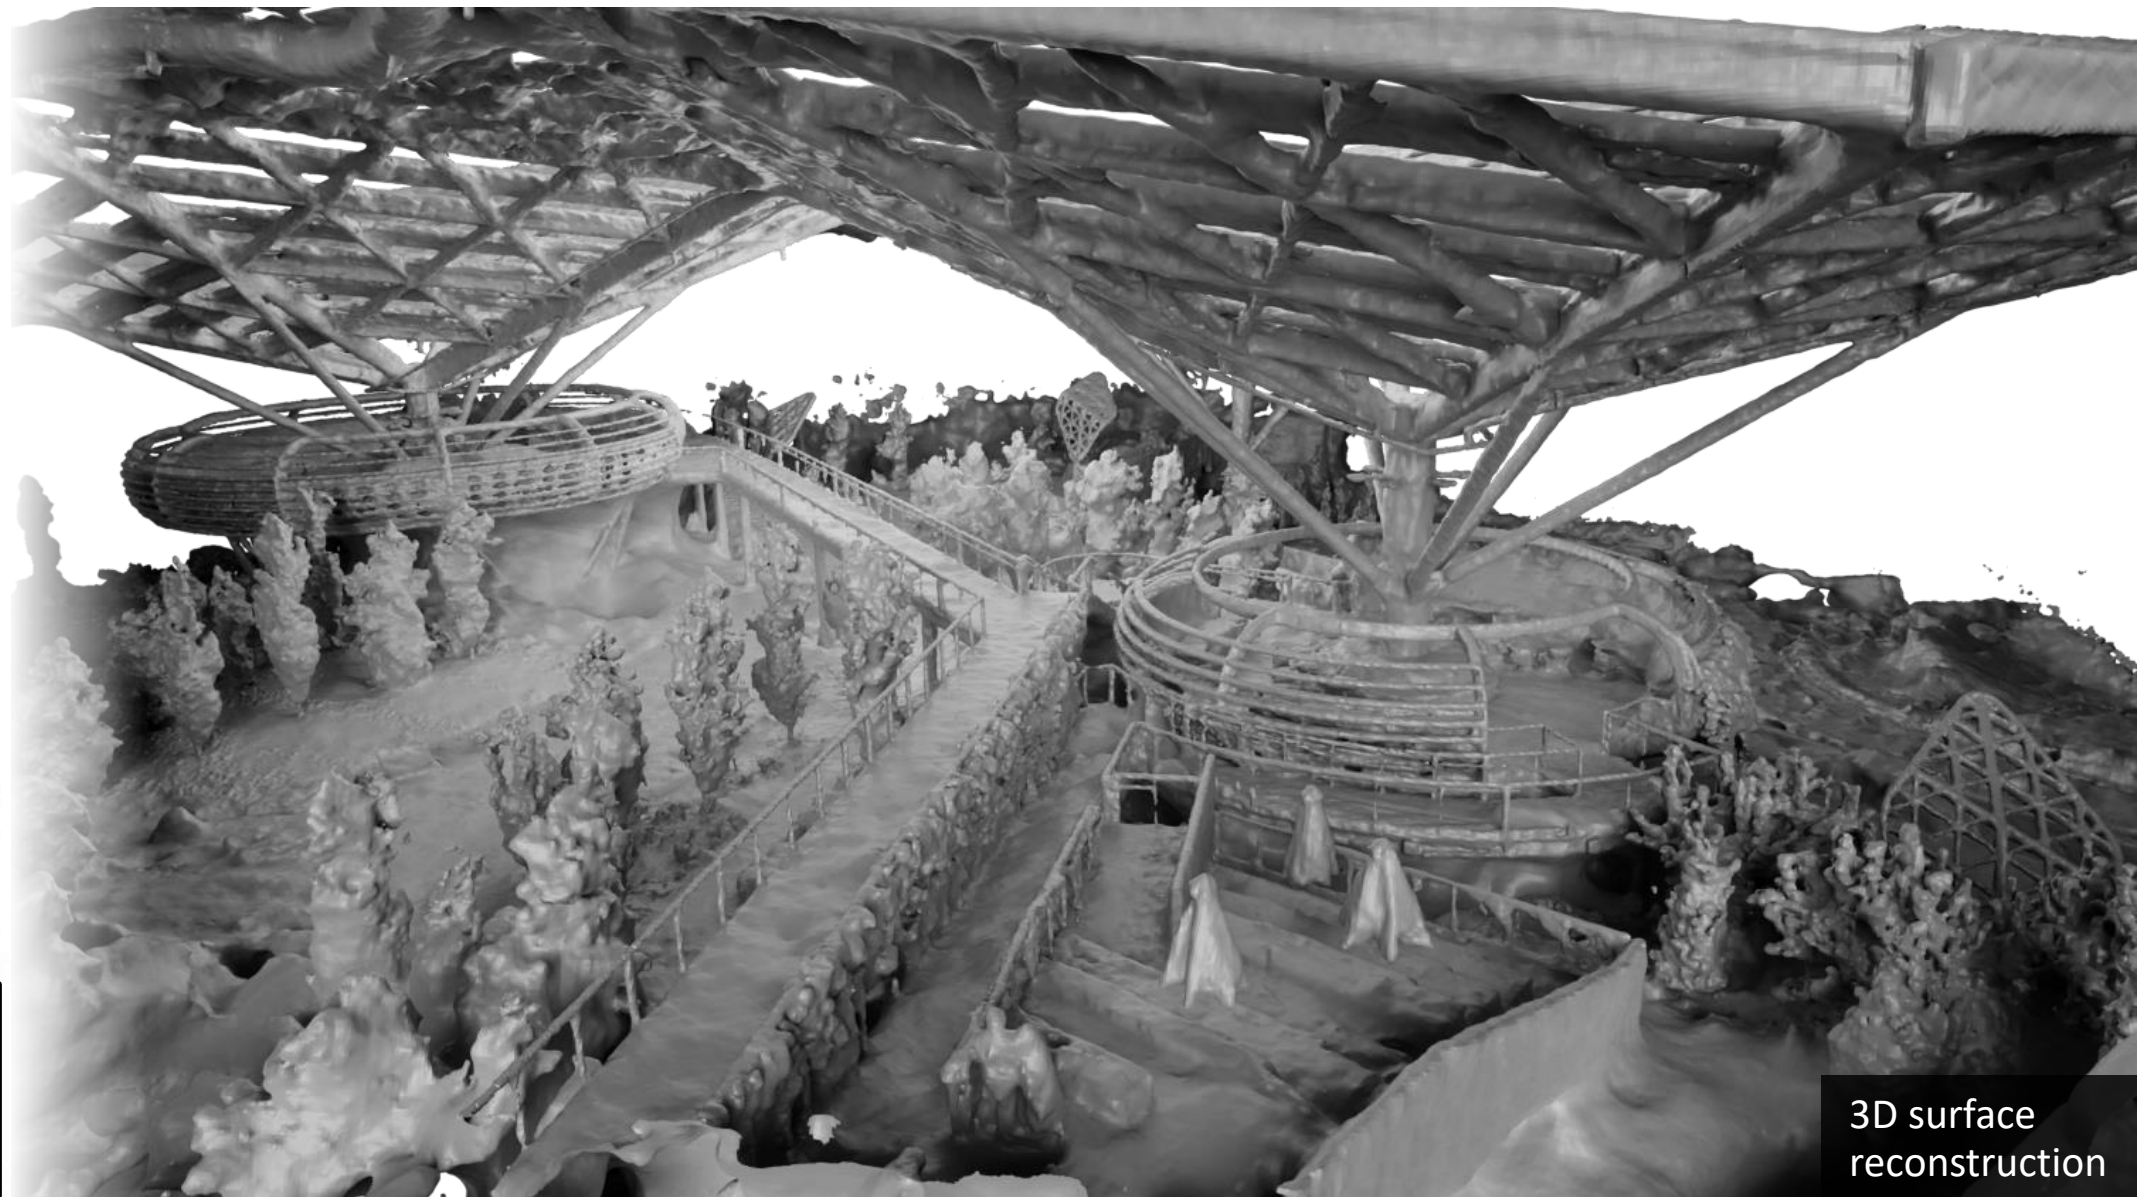

3D surface  
reconstruction

NVIDIA HQ Park

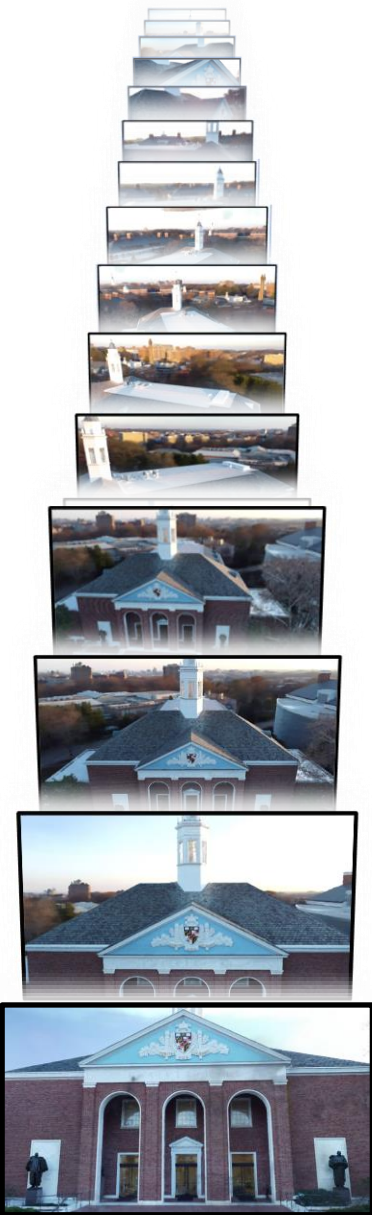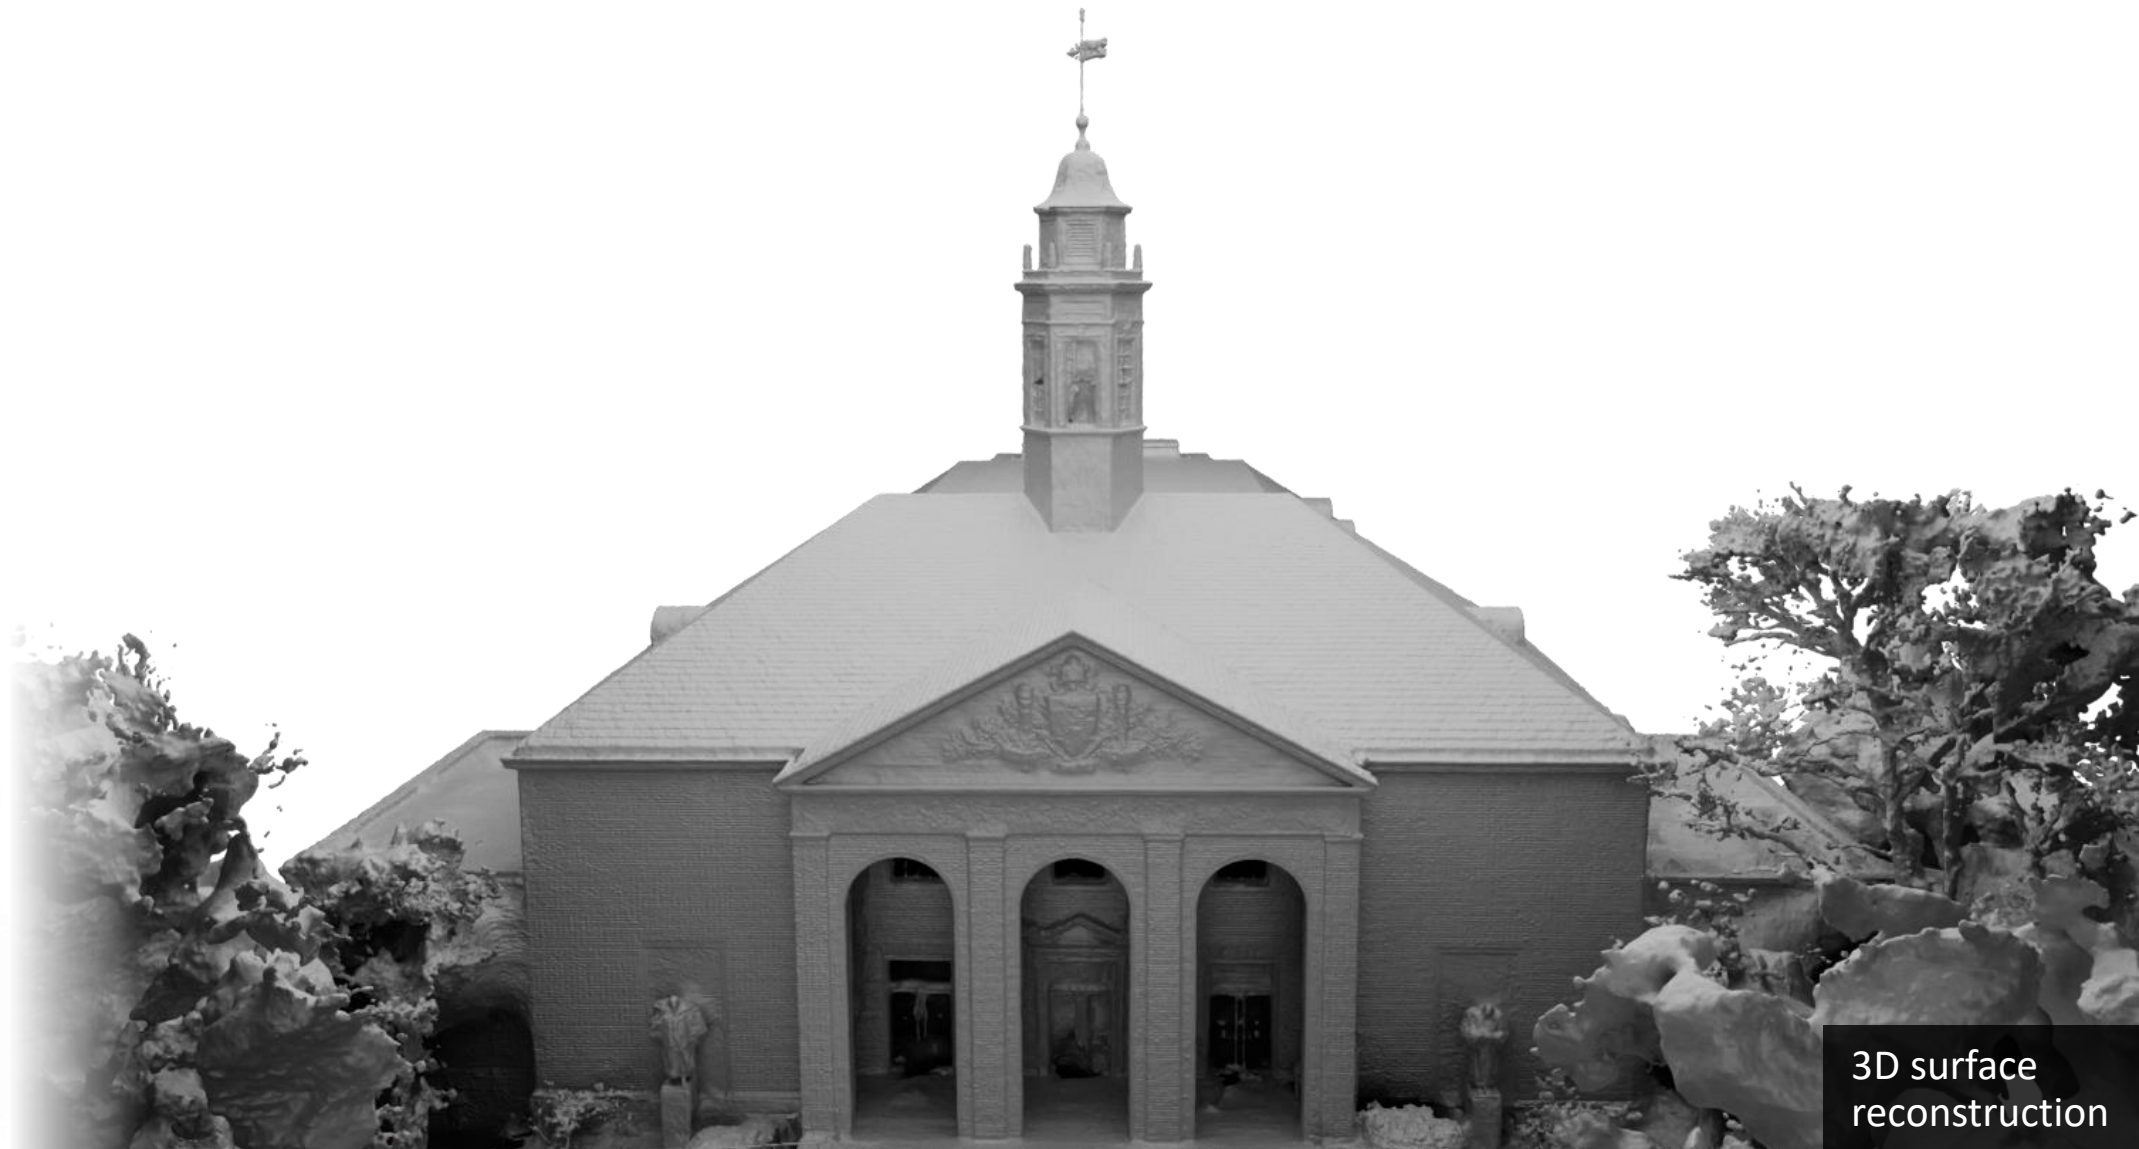

3D surface  
reconstruction

Johns Hopkins University
